# Supplementary material for: Why think step by step? Reasoning emerges from the locality of experience
Source: arXiv:2304.03843 source file (2023-11-02)
Supplement: Supplementary file 1 [file appendices_5-6_23.tex]

\appendix
\section{Full sample of training data}
\label{example_sample}
The following is an example of a sample from a local neighborhood of a Bayes net in string format, as used in training our models:
\begin{verbatim}
###
target: X5
X17=0
X92=0
X13=0
X52=1
X24=1
X26=1
X91=0
X36=0
X34=0
X12=1
X20=0
X5=1
\end{verbatim}
The full training set consists of $1,000,000$ samples like this concatenated together.

\section{Formatting estimators as prompts}
\label{example_prompts}

\subsection{Direct Prediction}

In direct prediction, we create a simple prompt that specifies the name and value of the observed variable, then states the name of the target variable. For example, if we wanted to estimate $p(X_2|X_1=0)$ we would create the following prompt:
\begin{verbatim}
###
target: X2
X1=0
X2=
\end{verbatim}
We would then take the softmax of the log-probabilities the language model assigns to `1' and `0' being the next token and use the probability of `1' as the estimate.

\subsection{Scaffolded Generation}

In scaffolded generation, we pre-compute a sequence of intermediate variables, then use the language model to estimate their values. For example, if we wanted to estimate $p(X_4|X_1)$ and we knew $X_2$ and $X_3$ were scaffold variables, we would start with the following prompt:
\begin{verbatim}
###
target: X4
X1=0
X2=
\end{verbatim}
We would then sample the next token from the language model and append it along with the next scaffold variable to the prompt. For example, if we got a value of $1$ from the language model, we would next give it the following prompt:
\begin{verbatim}
###
target: X4
X1=0
X2=1
X3=
\end{verbatim}
We repeat this process until all scaffold variables have values, then compute the probability assigned to the target variable at the end, in the same way we do for direct prediction. The final prompt we use to estimate the probability might look like this:
\begin{verbatim}
###
target: X4
X1=0
X2=1
X3=0
X4=
\end{verbatim}

We repeat this process 10 times to produce a Monte Carlo estimate over the values of the scaffold variables and average the probability assigned to the target variable over samples.

\subsection{Free Generation}

Free generation is similar to scaffolded generation, but we let the model choose which intermediate variables to instantiate, rather than just sample their values. For example, if we are trying to infer $p(X_4|X_1=0)$ we would first prompt it like this:
\begin{verbatim}
###
target: X4
X1=0
\end{verbatim}
We then sample the next two tokens from the model, which is exactly enough for one variable name. We add an equals sign, then sample the value of the variable in the same way as other conditions. For example, this might be what our prompt looks like after generating one intermediate variable and its value
\begin{verbatim}
###
target: X4
X1=0
X5=1
\end{verbatim}
We repeat this process until the model outputs the name of the target variable. At that point, we would have a prompt that might look like this
\begin{verbatim}
###
target: X4
X1=0
X5=1
X2=0
X7=0
X3=1
X4=
\end{verbatim}
We then extract the probability of the target variable in the standard way. Again, we average target variable probabilities over 10 samples of the intermediate variables.

\section{Pseudocode for data generation}
\label{data_gen_pseudocode}

This section contains pseudocode for the algorithms we use to generate Bayes nets and choose a subset of variables to include according to an observation distribution.

First, Algorithm~\ref{alg:net-generation} is used to create Bayes nets. This algorithm takes a number of nodes and edges and creates a directed acyclic graph by randomly adding edges between pairs of nodes. Next, it assigns conditional probability tables to the nodes given the values of their parents to create a Bayes net.

\input{algos/net-generation}

For each sample, we only show a subset of all the variables according to an observation distribution. Algorithm~\ref{alg:observation-distribution} shows the procedure we use to select which variables to display in a given sample. We first sample central variable $c$ and a distance $k$, then get all the variables within distance $k$ of $c$ in the graph. Next, we drop each variable with probability $0.2$. If any of the held-out pairs remain, we randomly remove one of them. In the wrong locality structure training conditions, we use a graph $G$ that does not correspond to the net from which our samples are drawn, but has the same variable names.

\input{algos/observation-distribution}

\section{Theoretical analysis} 
\label{theory_appendix}
In this section, we provide a theoretical analysis of chain of thought reasoning when the underlying data distribution can be represented as a directed chain. 
We prove that the risk minimizer will exhibit a ``reasoning gap''. 
\subsection{Assumptions} 
\paragraph{Assumption 1 (Factorization of data distribution)}
We assume that the joint distribution $p_d$ over $Y_1,Y_2, \ldots, Y_N$ factorizes as 
\begin{align*}
    p_d(Y_1, \ldots Y_N)= P(Y_1) \prod_{j=1}^N P(Y_{j+1} | Y_j)
\end{align*}
and that $Y_1, Y_2, \ldots, Y_N$ take support in some finite discrete set $\mathcal{X}$. 
\paragraph{Local observation distribution}
We assume that the joint distribution over the sequence, $p_{\text{obs}}(w_1, v_1, w_2, v_2, \ldots w_T, v_T)$, factorizes into products of independent local joint distributions consisting of pairs of variables and their values. 
For technical reasons, we symmetrize the observation distribution by imposing that it factorizes into one of two forms, with equal probability, depending on some initial condition.
\begin{align}
p(w_1, v_1, w_2, v_2) p(w_3, v_3, w_4, v_4 )  \ldots p(w_{T-1}, v_{T-1}, w_T, v_T) &&
\label{eq:joint_1}
\end{align}
or 
\begin{align}
% p_{\text{obs}}(w_{1:T}, v_{1:T})  & \\
p(w_1, v_1) p(w_2, v_2, w_3, v_3) \ldots p(w_{T-1}, v_{T-1}, w_T, v_T) && 
\label{eq:joint_2}
\end{align}
Without this assumption, the locations of the transitions between local neighborhoods are a deterministic function of the parity of $t$.
In real-world settings, we expect these transitions to occur irregularly.

We assume that each local neighborhood of random variables factorizes as follows
\begin{align*}
p_{\text{obs}}(w_{t-1}, v_{t-1}, w_t, v_t) = 
p_{\text{obs}}(v_t | w_{t-1}, v_{t-1}, w_t) p_{\text{obs}}(w_t | w_{t-1}) p_{\text{obs}}(v_{t-1} | w_{t-1}) p(w_{t-1})  
\end{align*}

The conditional distributions of the variable values are defined by $p_d$. 
In particular $p_\text{obs}(v_{t}|w_t, w_{t-1}, v_{t-1})$, the conditional distribution of the current variable value given the current variable identifier, previous variable identifier and its value, is specified by $p_d$.
Likewise, the conditional distribution $p_{\text{obs}}(v_{t-1} | w_{t-1})$ is given by the marginal distributions implied by $p_d$. 

Crucially, only adjacent random variables can appear together in a local neighborhood.
That is, all pairs of random variables within a local neighborhood are of the form $Y_i, Y_{i+1}$ for $i \in \{1, \ldots, N\}$. 
As a consequence, we will never see $Y_i$ and $Y_{j}$ together in a local neighborhood, whenever $|i-j| > 1$, which means we will never see samples from their joint distribution $p_d(Y_i, Y_j)$.
This key property of the observation distribution will induce a reasoning gap.
\subsection{Preliminaries}
We begin with a few propositions that will be useful in the main theorem.
The first proposition concerns the minimizer of the sum of two cross-entropy terms.
\begin{prop}
Let $R(q) = \mathbbm{E}_{p_{1}(x)}[-\log q(x)] + \mathbbm{E}_{p_{2}(x)}[-\log q(x)]$. Then $q^{*} = \arg\min R(q) = \frac{1}{2} p_1(x) + \frac{1}{2} p_2(x)$
\label{lemma_mixture}
\end{prop}
\begin{proof}
We assume the probability distributions are discrete but the argument generalizes to continuous random variables. 
The Lagrangian is given by
\begin{align}
    \mathcal{L}(q, \lambda) = -\sum_x p_1(x) \log q(x) + -\sum_x p_2(x) \log q(x) + \lambda_0 (\sum_x q(x) -1)
\end{align}

The first order conditions are 
\begin{align}
\frac{\partial{\mathcal{L}}}{\partial{q(x)}} = -\frac{p_1(x)}{q(x)} + -\frac{p_2(x)}{q(x)} + \lambda_0 = 0 && \\
\frac{\partial{\mathcal{L}}}{\partial{\lambda_0}} = 
\sum_x q(x) - 1 = 0 && \\ 
\end{align}
The first condition allows us to write $q(x) = \frac{p_1(x)+p_2(x)}{\lambda_0}$.
We can substitute this for $q$ into the other first order condition (\ie $q$ normalizes) to obtain
\begin{align*}
    \sum_x \frac{p_1(x)+p_2(x)}{\lambda_0} = 1
\end{align*}
This implies $\lambda_0 = 2$ and the desired result follows immediately.
\end{proof}

\subsection{Main Theorem}
Our main result is that the minimizer of the true risk under the observation distribution $p_{\text{obs}}$ and a cross-entropy loss function will exhibit a ``reasoning-gap''.
Our high level approach is to decompose the risk into cross-entropies across timesteps of the sequence. 
Expressing these cross entropies in terms of the $Y_j$'s will 
imply some conditions on the minimizer.
In the statement below, we will use the notation $x_t$ to denote elements of the sequence $w_1, v_1, \ldots, w_T, v_T$, where $x_t$ will be a variable identifier $w_t$ or a variable value $v_t$ depending on the index. 
We will let $x_0 \in \{0, 1\}$ index which factorization we use among Eq~\ref{eq:joint_1} and Eq~\ref{eq:joint_2}, with $x_0 = 0$ corresponding to the first factorization.
\begin{theorem}
Define the risk as a function of the distribution $q$ as follows
\begin{align}
    R(q) =\mathbbm{E}_{p_{\text{obs}}(x_{1:T}) }[\sum_{t} \log q(x_t | x_{1:t-1})]
\end{align}
Then $q^{*} = \arg \min_{q} R(q)$ satisfies the following properties. 
\begin{itemize}
    \item For all pairs of adjacent random variables $Y_i$ and $Y_j$, $q^{*}(Y_i|Y_j) = \frac{1}{2} p_{d}(Y_i|Y_j) + \frac{1}{2} p_{d}(Y_i)$. 
    \item $q^{*}(Y_n | Y_1) = p(Y_n)$. 
\end{itemize}
\label{main_theorem}
\end{theorem}

\begin{proof}

By conditioning on the initial condition $x_0$ and linearity of expectation, we can write 
\begin{align}
    R(q) = \sum_t -\mathbbm{E}_{p_{\text{obs}}(x_{0:T})}[\log q(x_t | x_{1:t-1})] \\
    = \frac{1}{2} \sum_t \mathbbm{E}_{p_{\text{obs}}(x_{1:t})}[-\log q(x_t | x_{1:t-1}) | x_0 = 0] +  \frac{1}{2} \sum_t \mathbbm{E}_{p_{\text{obs}}(x_{1:t})}[-\log q(x_t | x_{1:t-1}) | x_0 = 1]   &&  
    \label{eq: main}
\end{align}
By the law of iterated expectations, for any $t$, we can decompose each term where $x_t$ is a variable value as
\begin{align}
\mathbbm{E}_{p_{\text{obs}}(w_{1:t}, v_{1:t})}[-\log q(v_t | w_{1:t}, v_{1:t-1})] && \\
=  \mathbbm{E}_{p_{\text{obs}}(w_{1:t}, v_{1:t-1})} [\mathbbm{E}_{p_{\text{obs}}(v_t|w_{1:t}, v_{1:t-1})}[-\log q(v_t | w_{1:t}, v_{1:t-1})]]  && \\
= \sum_{w_{1:t}, v_{1:{t-1}}} \mathbbm{E}_{p_{\text{obs}}(v_t|w_{1:t}, v_{1:t-1})}[-\log q_t(v_t | w_{1:t}, v_{1:t-1})] p_{\text{obs}}(w_{1:t}, v_{1:t-1})
\label{eq:iterated_E}
\end{align}

When $x_0 = 0$, we have the following conditions that follow from the factorization assumptions that allow us to simplify the distributions that the expectations in Eq~\ref{eq:iterated_E} are taken with respect to.
When $t$ is even, we have that the last line is 
\begin{align}
\sum_{w_{1:t}, v_{1:{t-1}}} \mathbbm{E}_{p_{\text{obs}}(v_t|w_{t}, v_{t-1}, w_{t-1})}[-\log q(v_t | w_{1:t}, v_{1:t-1})] p_{\text{obs}}(w_{1:t}, v_{1:t-1})
\label{eq:conditionals_condition}
\end{align}
When $t$ is odd, we have
\begin{align}
\sum_{w_{1:t}, v_{1:{t-1}}} \mathbbm{E}_{p_{\text{obs}}(v_t|w_{t})}[-\log q(v_t | w_{1:t}, v_{1:t-1})] p_{\text{obs}}(w_{1:t}, v_{1:t-1})
\label{eq:marginals_condition}
\end{align}
We also have analogous statements for $x_0 = 1$.

Before proceeding further, we make two important observations. 
First, we can interpret the expectations that appear in Eq~\ref{eq:conditionals_condition} and Eq~\ref{eq:marginals_condition} as cross entropies between $q(\cdot)$ and $p(\cdot)$.
Second, since we condition on the current variable identifier and the previous variable identifier and its variable value, 
the distributions that appear in these cross entropy terms, 
are distributions wrt the random variables in the graphical model. 
That is $w_t = Y_i, w_{t-1} = Y_{j}$ for some $i, j \in \{1, \ldots, N\}$ s.t. $|i-j| = 1$.
For example, for even $t$, the cross entropy terms are between distributions of the form
$p_d(Y_i | Y_j = x')$ and $q(Y_i | Y_j = x', \ldots)$ for some $i, j \in \{1, \ldots, N\}$ and for some $x' \in \mathcal{X}$.

Consider $Y_i$, $Y_j$ and some fixed values for the preceding variable identifiers and values (\ie $Y_j = x_j' \in \mathcal{X}, Y_k = x_k' \in \mathcal{X}, \ldots$). 
We combine all cross-entropy terms in $R(q)$ that involve $q(Y_i | Y_j = x_j', Y_k = x_k', \ldots)$.
By the symmetry of the observation distribution, for any adjacent pair of nodes, we can find exactly two terms of this form in Eq~\ref{eq: main}; we can simply take one term from each of the two sums. 
Reading off Eq~\ref{eq:iterated_E}, we see these terms are
\begin{align}
    \mathbbm{E}_{p(Y_i)}[-\log q(Y_i | Y_j = x_j', Y_k = x_k', \ldots)] p(w_t = Y_i, v_{t-1} = x_j', w_{t-1} = Y_j, w_{t-2} = Y_k, \ldots)
\end{align}
\begin{align}
    \mathbbm{E}_{p(Y_i | Y_j)}[-\log q(Y_i | Y_j = x_j', Y_k = x_k', \ldots)] p(w_t = Y_i, v_{t-1} = x_j', w_{t-1} = Y_j, w_{t-2} = Y_k, \ldots)
\end{align}

Notice that these are expectations wrt $p(Y_i)$ or $p(Y_i|Y_j)$.
By an application of Proposition~\ref{lemma_mixture},
the sum of these two terms is minimized by taking $q^{*}(Y_i | Y_j = x_j', Y_k = x_k', \ldots) = \frac{1}{2} p(Y_i) + \frac{1}{2} p(Y_i | Y_j)$.
The result holds for any $i, j$, with $|i-j| > 1$ and any set of predecessors. 
Therefore, we have that $q^{*}(Y_i | Y_j) = \frac{1}{2} p(Y_i) + \frac{1}{2} p(Y_i | Y_j)$, for all adjacent pairs.

Finally, we consider non-adjacent pairs $Y_i$ and $Y_j$.
By construction, terms of the form $\log q(Y_i | Y_j, \ldots)$ or $\log q(Y_n | Y_1, \ldots)$ only appear inside cross entropy terms that are expectations with respect to $p(Y_i)$ or $p(Y_j)$ respectively.
Therefore, we have $q^{*}(Y_i | Y_j) = p(Y_i)$ and $q^{*}(Y_j | Y_i) = p(Y_j)$.
% Finally, we consider the pairs $Y_1$ and $Y_n$.
% By construction, terms of the form $\log q(Y_1 | Y_n, \ldots)$ or $\log q(Y_n | Y_1, \ldots)$ only appear inside cross entropy terms that are expectations with respect to $p(Y_1)$ or $p(Y_N)$.
% Therefore, we have $q^{*}(Y_n | Y_1) = p(Y_n)$ and $q^{*}(Y_1 | Y_n) = p(Y_1)$.
\end{proof}

As a simple consequence of convexity and Theorem~\ref{main_theorem}, we can show that for all pairs besides the held-out pairs, $q^{*}$ is closer in KL-divergence to the true conditional probability distributions than the marginals. 
\begin{corollary}
For all pairs $Y_i$ and $Y_{i+1}$ that 
\begin{align*}
    KL[p(Y_{i+1}|Y_i)||q^{*}(Y_{i+1} | Y_{i}) ] \leq KL[p(Y_{i+1}|Y_i) || p(Y_i)]
\end{align*}
\begin{proof}
We use the fact that
$KL[\lambda p_1 + (1-\lambda) p_2 || \lambda q_1 + (1-\lambda) q_2] \leq \lambda KL[p_1||q_1] + (1-\lambda) KL[p_2||q_2]$ and the optimality condition we obtained for $q^{*}(Y_{i+1} | Y_i) = \frac{1}{2} p(Y_{i+1}) + \frac{1}{2} p(Y_{i+1} | Y_i)$.
Let us take $p_1 = p_2 = p(Y_{i+1}|Y_i)$ and $q_1 = p(Y_{i+1}), q_2 = p(Y_{i+1}|Y_i)$. 

\begin{align}
KL[p(Y_{i+1}|Y_i)||q^{*}(Y_{i+1}|Y_i)] && \\
= KL[p(Y_{i+1}|Y_i)||\frac{1}{2} p(Y_{i+1}) + \frac{1}{2} p(Y_{i+1} | Y_i)] && \\
\leq 
\frac{1}{2} KL[P(Y_{i+1}|Y_i)||P(Y_{i+1})] 
+ \frac{1}{2} KL[p(Y_{i+1}|Y_i) || p(Y_{i+1}|Y_i)] && \\
\leq KL[P(Y_{i+1}|Y_i)||P(Y_i)] &&
\end{align}
The last line follows from the non-negativity of KL and the fact that $KL[p(Y_{i+1}|Y_i) || p(Y_{i+1}|Y_i)] = 0$.

\end{proof}
\end{corollary}

In the following corrollary we will show that squared bias of the scaffolded generation estimator is less than the squared bias of the direct estimator.
% However, assuming that $q^{*}$ matches the exact conditionals of $p$, which is true in practice, the following corollary will show that this limitation poses no fundamental complications.
\begin{theorem}
% Define the scaffolded distribution $q^{*}_{SG}(Y_j | Y_i)$ as the distribution obtained by marginalizing out intermediate variables $Y_{i+1}, \ldots Y_{j-1}$, using the estimates of the local conditional probabilities $q^{*}(Y_i|Y_{i-1})$. 
% \begin{align*}
%     q^{*}_{SG}(Y_j = y_j | Y_i= y_i) = \sum_{Y_{j-1}} \ldots \sum_{Y_{i+1}} q^{*}(Y_j | Y_{j-1}) \prod_{k= i+1}^{j-1} q^{*}(Y_k|Y_{k-1}) 
% \end{align*}
% Define the scaffolded estimator as the Monte Carlo approximation to the scaffolded distribution (\ie all intermediate local distribution are sampled from $q^{*}(Y_j | Y_{j-1}$))
% \begin{align*}
%     \hat{q}_{SG}(Y_n = y_n|Y_1=y_1) = \frac{1}{N} \sum_{i=1}^N \mathbbm{1}_{\{Y_n^{(i)} = y_n\}} && Y_n \sim q_{SG}^{*}(Y_n|Y_1 = y_1)    
% \end{align*}
% Define the direct distribution as the Monte Carlo approximation
% \begin{align*}
%     q^{*}_{DE}(Y_j | Y_i) = q^{*}(Y_j | Y_i)
% \end{align*}
% and the direct estimator as
% \begin{align*}
%     \hat{q}_{DE}(Y_n = y_n|Y_1=y_1) = \frac{1}{N} \sum_{i=1}^N \mathbbm{1}_{\{Y_n^{(i)} = y_n\}} && Y_n \sim q_{DE}^{*}(Y_n|Y_1 = y_1)    
% \end{align*}

For all $y_i, y_j \in \mathcal{X}$ with $|i-j|>1$,
\begin{align*}
    |\mathbbm{E}_{Y_n \sim  q^{*}_{S}(Y_i = y_i| Y_j = y_j)}[\hat{q}^{*}_{S}(Y_i = y_i)] - p(Y_i = y_i | Y_j = y_j)
|^2 && \\ 
    < 
    |\hat{q}^{*}_{D}(Y_i = y_j)-p(Y_i = y_i | Y_j = y_j)|^2
\end{align*}
% \begin{align*}
%     |\mathbbm{E}_{Y_n \sim  q^{*}_{SG}(Y_n|Y_1)}[\hat{q}^{*}_{SG}(Y_n = y_n)] - p(Y_n = y_n | Y_1 = y_1)
% |^2 && \\ 
%     < 
%     |\mathbbm{E}_{Y_n \sim  q^{*}_{\text{DE}}(Y_n|Y_1)}[\hat{q}^{*}_{DE}(Y_n = y_n)]
%     - p(Y_n = y_n | Y_1 = y_1)|^2
% \end{align*}
\label{ref:estimator_bias_thm}
\end{theorem}
\begin{proof}
We will calculate both sides of the inequality.
We begin by showing that $\mathbbm{E}_{Y_n \sim  q^{*}_{S}(Y_n|Y_1)}[\hat{q}^{*}_{S}(Y_n=y_n|Y_1=y_1)]  = \lambda p(Y_n|Y_1) + (1-\lambda)p(Y_n)$ for some $\lambda \in (0, 1)$.
For the scaffolded estimator, by linearity of expectation, it suffices to consider the expected value of a single term in the sum. 
Furthermore, we prove this result for the  case where $Y_i = Y_3$ and $Y_j = Y_1$ and then the desired result follows from induction and the stationarity of the sequence.
\begin{flalign*}
\mathbbm{E}_{y_2 \sim q^{*}_{\text{S}}(Y_{2}|Y_1)}[q^{*}(Y_3 = y_3 | Y_2 = y_2)] && \\
= \sum_{y_2} q^{*}(Y_3 = y_3 | Y_2 = y_2) q^{*}(Y_2 = y_2 | Y_1 = y_1) && \\
= \mathbbm{E}_{y_2 \sim q^{*}_{\text{S}}(Y_{2}|Y_1)}[\frac{1}{2}p(Y_{3} = y_3 |Y_{2} = Y2) + \frac{1}{2}p(Y_3=y_3)] && \text{by Theorem \ref{main_theorem}} \\
= \frac{1}{2}p(Y_3) + \mathbbm{E}_{y_2 \sim q^{*}_{\text{S}}(Y_{2}|Y_1)}[\frac{1}{2}p(Y_{3}|Y_{2})] && \\
= \frac{1}{2}p(Y_3=y_3) + \frac{1}{4} \sum_{y_2} p(Y_3 = y_3 | Y_2 = y_2) p(Y_2=y_2|Y_1=y_1) + \frac{1}{4} \sum_{y_2} p(Y_3 = y_3 | Y_2=y_2) p(Y_2=y_2) && \\
= \frac{1}{2} p(Y_3=y_3) + \frac{1}{4} p(Y_3=y_3|Y_1=y_1) + \frac{1}{2} p(Y_3=y_3) && \\
= \frac{3}{4}p(Y_3=y_3) + \frac{1}{4} p(Y_3=y_3|Y_1=y_1)
\end{flalign*}    
\end{proof}
% \begin{align}
%     \mathbbm{E}_{q^{*}_{\text{SG}(Y_{3}|Y_1)}}[\mathbbm{1}_{\{Y_3 = y_3\}}] && \\
%     = \mathbbm{E}_{q^{*}_{\text{SG}(Y_{2}|Y_1)}}[\mathbbm{E}_{q^{*}_{\text{SG}(Y_{3}|Y_{2})}}[\mathbbm{1}_{\{Y_3 = y_3\}}]] && \\
%     = \mathbbm{E}_{q^{*}_{\text{SG}(Y_{2}|Y_1)}}[\frac{1}{2}p(Y_{3}|Y_{2}) + \frac{1}{2}p(Y_3)] && \text{by Theorem \ref{main_theorem}} \\
%     = \frac{1}{2}p(Y_3) + \mathbbm{E}_{q^{*}_{\text{SG}(Y_{2}|Y_1)}}[\frac{1}{2}p(Y_{3}|Y_{2})] && \\
%     = \frac{1}{2}p(Y_3) + \frac{1}{4} \sum_{Y_2} p(Y_3 = y_3 | Y_2) p(Y_2|Y_1) + \frac{1}{4} \sum_{Y_2} p(Y_3 = y_3 | Y_2) p(Y_2) && \\
%     = \frac{1}{2} p(Y_3) + \frac{1}{4} p(Y_3|Y_1) + \frac{1}{2} p(Y_3) && \\
%     = \frac{3}{4}p(Y_3) + \frac{1}{4} p(Y_3|Y_1)
% \end{align}    
% \end{proof}
Importantly, the expected value is a convex combination of the marginal and conditional probabilities. 
Before proceeding, we make a few additional comments.
In the setting we consider, the bias of the scaffolded estimator compounds with the length of the chain since there is bias in the estimates of local conditional probabilities.
In practice, the scaffold lengths are small and $q^{*}$ estimates the local conditional probabilities well; if $q^{*}$ matches the exact conditionals of $p$, which is close to the situation in practice, then we can show the scaffolded estimator is unbiased.

The bias of direct estimator can be computed as $|p(Y_i=y_i)-p(Y_i = y_i | Y_j = y_j)|^2$.
% Since $q^{*}(Y_i | Y_j) = p(Y_i)$, we have that
% \begin{align}
%     \mathbbm{E}_{Y_n \sim  q^{*}_{DE}(Y_n|Y_1)}[\mathbbm{1}_{\{Y_n = y_n\}}] = 
%     p(Y_n)
% \end{align}
% \begin{align}
%     \mathbbm{E}_{Y_n \sim  q^{*}_{DE}(Y_n|Y_1)}[\mathbbm{1}_{\{Y_n = y_n\}}] = 
%     p(Y_n)
% \end{align}
Finally, we show that these results imply the desired inequality.
By the previous results, $\mathbbm{E}_{Y_n \sim  q^{*}_{S}(Y_n|Y_1)}[\hat{q}^{*}_{S}(Y_n=y_n|Y_1=y_1)]  = \lambda p(Y_n|Y_1) + (1-\lambda)p(Y_n)$ for some $\lambda \in (0, 1)$.

\begin{align*}
|\mathbbm{E}_{y_i \sim  q^{*}_{S}(Y_i|Y_j=y_j)}[\hat{q}^{*}_{S}(Y_i|Y_j=y_j)] - p(Y_i = y_i | Y_j = y_j)|^2 && \\
= |\lambda p(Y_i = y_i | Y_j = y_j) + (1-\lambda)p(Y_i = y_i) - p(Y_i = y_i | Y_j = y_j)|^2 && \\
= |\lambda p(Y_i = y_i | Y_j = y_j) + p(Y_i = y_i)-\lambda p(Y_i = y_i) - p(Y_i = y_i | Y_j = y_j)|^2 && \\
= |(\lambda-1)p(Y_i = y_i | Y_j = y_j) + (1-\lambda)p(Y_i = y_i)|^2 && \\
= (1-\lambda)^2|(p(Y_i = y_i) - p(Y_i = y_i | Y_j = y_j)|^2 && \\
<
|p(Y_i = y_i)- p(Y_i = y_i | Y_j = y_j)|^2
\end{align*}

% old
% \begin{align*}
% |\mathbbm{E}_{y_i \sim  q^{*}_{SG}(Y_i|Y_j=y_j)}[\hat{q}^{*}_{S}(Y_i|Y_j=y_j)] - p(Y_i = y_i | Y_j = y_j)|^2 && \\
% = |\lambda p(Y_i = y_i | Y_j = y_j) + (1-\lambda)p(Y_i = y_i) - p(Y_i = y_i | Y_j = y_j)|^2 && \\
% = |\lambda p(Y_i = y_i | Y_j = y_j) + p(Y_i = y_i)-\lambda p(Y_i = y_i) - p(Y_i = y_i | Y_j = y_j)|^2 && \\
% = |(\lambda-1)p(Y_i = y_i | Y_j = y_j) + (1-\lambda)p(Y_i = y_i)|^2 && \\
% = (1-\lambda)^2|(p(Y_i = y_i) - p(Y_i = y_i | Y_j = y_j)|^2 && \\
% <
% |\mathbbm{E}_{y_i \sim  q^{*}_{\text{DE}}(Y_i|Y_j=y_j)}[\hat{q}^{*}_{D}(Y_i = y_i|Y_j=y_j)]
%     - p(Y_i = y_i | Y_j = y_j)|^2
% \end{align*}

% \begin{align*}
% |\mathbbm{E}_{Y_n \sim  q^{*}_{SG}(Y_n|Y_1)}[\hat{q}^{*}_{SG}(Y_n = y_n)] - p(Y_n = y_n | Y_1 = y_1)|^2 && \\
% = |\lambda p(Y_n = y_n | Y_1 = y_1) + (1-\lambda)p(Y_n = y_n) - p(Y_n = y_n | Y_1 = y_1)|^2 && \\
% = |\lambda p(Y_n = y_n | Y_1 = y_1) + p(Y_n = y_n)-\lambda p(Y_n = y_n) - p(Y_n = y_n | Y_1 = y_1)|^2 && \\
% = |(\lambda-1)p(Y_n = y_n | Y_1 = y_1) + (1-\lambda)p(Y_n = y_n)|^2 && \\
% = (1-\lambda)^2|(p(Y_n = y_n) - p(Y_n = y_n | Y_1 = y_1)|^2 && \\
% <
% |\mathbbm{E}_{Y_n \sim  q^{*}_{\text{DE}}(Y_n|Y_1)}[\hat{q}^{*}_{DE}(Y_n = y_n)]
%     - p(Y_n = y_n | Y_1 = y_1)|^2
% \end{align*}
% \begin{corollary}
% Suppose $Y_{i} \sim q^{*}(Y_n|Y_1)$. 
% Let the direct estimator of the conditional probability be defined as: 
% \begin{align*}
%     \hat{q_{DE}}(Y_n = y_n|Y_1=y_1) = \frac{1}{N} \sum_{i=1}^N \mathbbm{1}_{\{Y_n^{(i)} = y_n\}} && Y_n \sim q_{DE}^{*}(Y_n|Y_1 = y_1)    
% \end{align*}
% \end{corollary}
% \begin{proof}
